# Supplementary material for: Metal-chalcogen bond-length induced electronic phase transition from semiconductor to topological semimetal in ZrX$_2$ (X = Se and Te)
Source: arXiv:1907.03987 source file (2019-07-09)
Supplement: Supplementary file 1 [file ZrX2-Suppl..pdf]

# Metal-chalcogen bond-length induced electronic phase transition from semiconductor to topological semimetal in $ZrX_2$ ($X = Se$ and $Te$)

I. Kar,[1] Joydeep Chatterjee,[1] Luminita Harnagea,[2] Y. Kushnirenko,[3] A. V. Fedorov,[3] Deepika Shrivastava,[1] B. Büchner,[3] P. Mahadevan,[1] and S. Thirupathaiah[1,3,*]

[1] *Condensed Matter Physics and Material Science Department, S N Bose National Centre for Basic Sciences, 700106, India*

[2] *Indian Institute of Science Education and Research, Dr. Homi Bhabha Road, Pune, Maharashtra-411008, India*

[3] *Leibniz Institute for Solid State Research, IFW Dresden, D-01171 Dresden, Germany*

( Dated: July 9, 2019)

* setti@bose.res.in

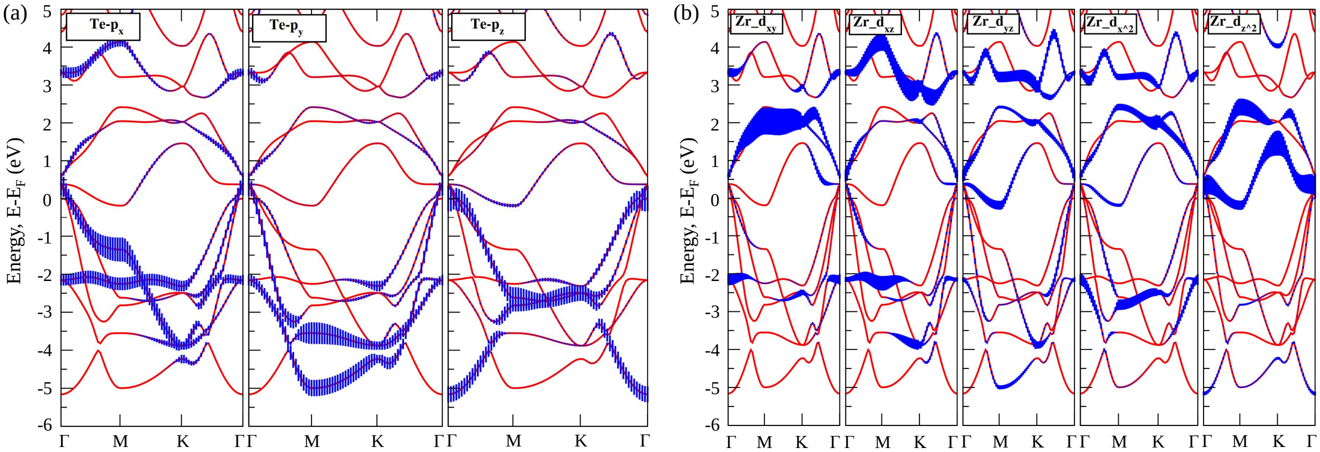


Figure 1. Orbital resolved calculated band structure of $ZrTe_2$ without SOC for (a) Te $p$ states (b) Zr $d$ states.

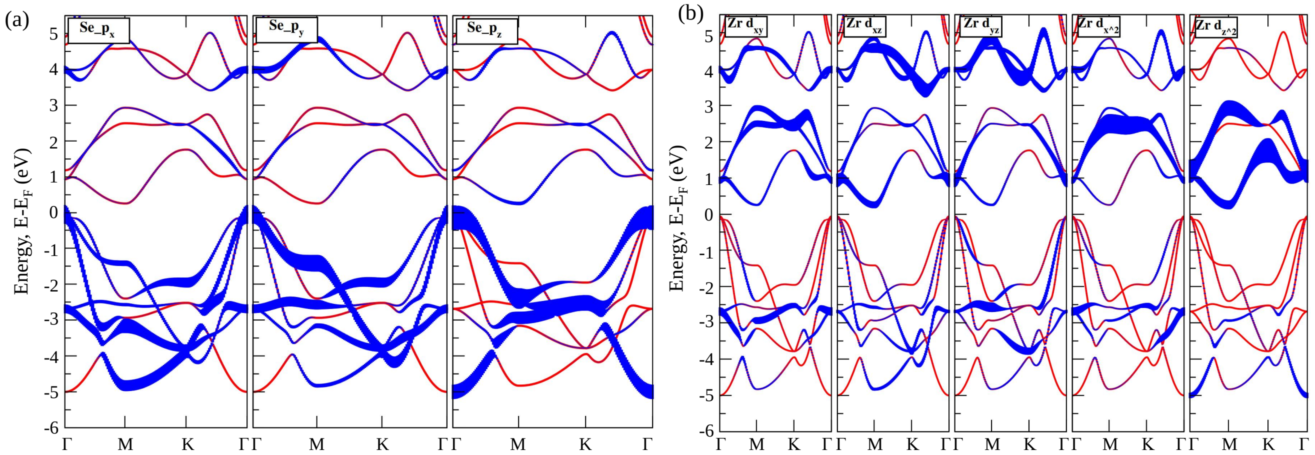


Figure 2. Orbital resolved calculated band structure of $ZrSe_2$ without SOC for (a) Se $p$ states (b) Zr $d$ states.

**$ZrSe_2$ :**

**Optimized lattice vectors of $ZrSe_2$**

| | | |
|---|---|---|
| 3.7352 | 0.0000 | 0.0000 |
| -1.8676 | 3.2348 | 0.0000 |
| 0.0000 | 0.0000 | 6.2058 |

Onsite energies of $ZrSe_2$

| Atom | Orbital | Onsite energies $\varepsilon_i$ | Δ (eV) |
|---|---|---|---|
| Zr | $d_{z^2}$ | 4.21 | 2.350 |
| | $d_{xz}$ | 5.00 | |
| | $d_{yz}$ | 4.93 | |
| | $d_{x^2}$ | 4.49 | |
| | $d_{xy}$ | 4.49 | |
| Se1 | $p_z$ | 1.78 | |
| | $p_x$ | 1.86 | |
| | $p_y$ | 1.83 | |
| Se2 | $p_z$ | 1.78 | |
| | $p_x$ | 1.86 | |
| | $p_y$ | 1.83 | |

**$ZrTe_2$:**

**Optimized lattice vectors of $ZrTe_2$**

| | | |
|---|---|---|
| 3.9086 | 0.0000 | 0.0000 |
| -1.9543 | 3.3849 | 0.0000 |
| 0.0000 | 0.0000 | 6.7488 |

Onsite energies of $ZrTe_2$

| Atom | Orbital | Onsite energies $\varepsilon_i$ | Δ (eV) |
|---|---|---|---|
| Zr | $d_{z^2}$ | 6.24 | 2.175 |
| | $d_{xz}$ | 7.04 | |
| | $d_{yz}$ | 7.04 | |
| | $d_{x^2}$ | 6.51 | |
| | $d_{xy}$ | 6.51 | |
| Te1 | $p_z$ | 3.95 | |
| | $p_x$ | 4.06 | |
| | $p_y$ | 4.06 | |
| Te2 | $p_z$ | 3.95 | |
| | $p_x$ | 4.06 | |
| | $p_y$ | 4.06 | |

Figure 3. Optimized lattice parameters obtained from the DFT calculations using PBE approximation with dispersion corrections included. Corresponding onsite energies obtained from a mapping of DFT band dispersions onto a tight binding model have been given. Charge transfer energy $= E(d_{z^2})$-$E(p_z)$ also has been given.
